# Supplementary material for: SignLLM: Sign Language Production Large Language Models
Source: arXiv:2405.10718 source file (2025-04-30)
Supplement: Supplementary file 1 [file suppl_more_intro.tex]

\section{More Introduction}

% Proposed method
In this paper, we introduce the first large-scale model for bilingual sign language production and construct the largest standardized bilingual sign language dataset to date. Initially, we propose a Multi-Language Switching Framework (MLSF) for \ac{slp}, based on state-of-the-art work in related fields. This framework dynamically incorporates an increasing number of encoders-decoders, enabling concurrent production of diverse sign languages. With two pipelines, text2gloss2pose and text2pose, it facilitates the production of a variety of sign language skeletal postures.

% MLSF part
In order to enable the MLSF framework to support static single-group coders and decoders for multilingual sign language production, we have developed two enhanced modules specifically improved for non-dynamic multilingual production and large-scale data training strategies. To avoid overfitting and redundant training caused by large datasets, we have for the first time introduced a novel loss based on the concept of reinforcement learning in sign language. This can reasonably prevent the problem of lengthy training times caused by large datasets, and also make it possible to seriously learn sign languages that are not known.

% Prompt2Sign part
In order to train \ourLLMmethodName{} with our new framework, we have constructed a new dataset named Prompt2Sign. It currently primarily sources from How2Sign and PHOENIX-14T, and we have spent several months recreating and optimizing them according to our model standards, reducing the space they occupy to one-tenth of their original size without any loss of data. To equip \ourLLMmethodName{} with conversational capabilities, we have synthesized 40,000 snippet prompts, making Prompt2Sign the most suitable dataset for large models of sign language. It can also rewrite prompts to enhance the robustness of large models, making it the largest dataset for future training of large sign language models.
