# Supplementary material for: SignLLM: Sign Language Production Large Language Models
Source: arXiv:2405.10718 source file (2025-04-30)
Supplement: Supplementary file 2 [file suppl_more_method.tex]

\section{More Details of Methodology}

\subsection{Motivation} \label{sec:Motivation}

For multilingual sign language production and large language models, the challenges lie in the convenient switching or expansion of the types of sign language, and the availability of a sufficiently large amount of high-quality data. Accordingly, we propose a new MLSF framework to handle the case of shared parameters among various sign languages. We incorporate two new components, "Text2LangGloss" and "Priority Learning Channel", to separately address the issues of multiple sign languages using a set of parameters (based on learning from prompt words) and overfitting as well as prolonged training time with large-scale data. We have a reinforcement learning-based loss adapted to the new model, which expands the possibilities of sign language production.

\subsection{Our innovative BSLP}

\paragraph{Multi-Language Switching Framework}

The profundity manifest in the presented piece of code lies in its capacity for dynamic language adaptation in the context of an encoder-decoder framework, specifically tailored for sign languages. Utilizing Python dictionaries, this paradigm ingeniously allows different encoders and decoders pertaining to distinct languages to be introduced into the model.

Given the set of encoders $\mathcal{E} = \{\epsilon_1, \epsilon_2, \ldots, \epsilon_n\}$ and decoders $\mathcal{D} = \{\delta_1, \delta_2, \ldots, \delta_n\}$ corresponding to $n$ languages, the novel implementation specifically assigns an encoder and decoder out of $\mathcal{E}$ and $\mathcal{D}$, respectively, determined by the language $\mathcal{L}$.
The ascription operation is formalized as $\text{Enc}_{\mathcal{L}} = \mathcal{E}_\mathcal{L}$ and $\text{Dec}_{\mathcal{L}} = \mathcal{D}_\mathcal{L}$, effectively setting the language-specific components for the current run.

The fortification of this framework provides an unequivocal advantage of incorporating a wide array of sign languages into the model, enhancing the flexibility and scalability, while also cutting down on extraneous computational cost typically associated with maintaining separate models for each language. Consequently, this dynamic substitution underscores the model's ability to be a universally applicable abstract sign language translation model.

The crowning achievement lies not only in the dexterity of the code but also in the mathematical robustness of the approach itself. In a sense, it placidly embeds a discrete 'choice' function $\chi: \mathcal{L} \to \mathcal{E} \times \mathcal{D}$ mapping languages to a tuple of encoder-decoder pairs, leveraging the power of modern functional programming paradigms alongside the inarguable efficacy of the foundational mathematical structures.
This gaping stride resonates well with the tenets of a cutting-edge approach to machine learning, focusing equally on the mathematical grants of versatility and the practical considerations of optimality and computational efficiency.

\paragraph{Text2LangGloss}

In the realm of sign language generation, Gloss plays a pivotal role. Acting as a textual depiction of sign language gestures, Gloss forms a crucial intermediary in a text-to-gloss (T2G) model. We propose an improvement to this model, which encompasses the attachment of an additional linguistic attribute to each Gloss during the parsing and tokenizing stages. For instance, a typical Gloss token "xxx" can be modified to "ASL\_xxx", which adds an element of conditional input to sign language generation.

The advantages of employing this method are manifold. Initially, it facilitates a single model to concurrently manage parameters for numerous languages, thereby nullifying the necessity for alternating between platforms or models. This alleviates a prominent intricacy associated with linguistics—overlapping of the semantic essence of words across different languages, which may lead to potential ambiguity. Our LangGloss as a conditional input helps to stratify these overlaps, subsequently significantly diminishing the chance of model errors.

Moreover, our approach augments the model robustness. In an instance where all Gloss tokens start with the prefix "ASL\_" and a single "GSL\_" token is inaccurately included, our refined model recognizes this token as an error given the pre-set conditions, thereby substantially mitigating the likelihood of errors, potentially by a factor of 10 or even 100. Therefore, our Text2LangGloss method introduces a strategic and streamlined solution for sign language generation across various languages.

Given a spoken language sequence, it is initially converted into a sequence of gloss tokens, each supplemented with its corresponding linguistic attribute, forming a LangGloss sequence. As such, a source sequence denoted by $\mathcal{X} = (x_{1},...,x_{\mathcal{T}})$ in the spoken language is mapped to a LangGloss sequence indicated by $\mathcal{Z} = (L_{1}z_{1},...,L_{\mathcal{W}}z_{\mathcal{W}})$, wherein $L_{i}$ refers to the linguistic attribute of each gloss token and $\mathcal{W}$ implies the total count of LangGloss tokens.

The equations are defined as follows:

\begin{equation}
\label{eq:T2LG_encoder}
    f_{t} = E_{T2LG}(x_{t} | x_{1:t-1})
\end{equation}

\begin{equation}
\label{eq:T2LG_decoder}
    g_{w+1} = D_{T2LG}(g_{w}  | g_{1:w} , f_{1:\mathcal{T}})
\end{equation}

Here, $f_{t}$ and $g_{w}$ denote the encoded source and target tokens respectively, with $g_{0}$ initialized as the encoding of the special $\mathrm{<bos>}$ token. The LangGloss tokens are allocated based on the maximum decoder output value, i.e., $ z_{w} = \operatorname*{argmax}_{i} (g_{w})$, a procedure that continues until the special $\mathrm{<eos>}$ token is predicted. 

Ultimately, this framework empowers the model to maintain parameters for various sign languages concurrently, minimizing any potential ambiguity during prediction and enhancing the robustness of the system.

\paragraph{Priority Learning Channel} 

The cornerstone of our methodology is the introduction of a Priority Learning Channel (PLC) that inherently directs the model's attention towards high-reward data samples. The principal hypothesis underwriting this approach is that such targeted learning would not only expeditiously aid in model convergence but would also boost the model's overall performance. 

We define the reward of each data sample as the absolute difference between the model's prediction and the actual target, mathematically denoted as $r(i) = \|y_i-\hat{y}_i\|$. These rewards are converted into sampling probabilities for each data sample according to 
\begin{equation}
 P(i) = \frac{ r(i)^\eta}{\sum_{j \in S} r(j)^\eta}, 
\end{equation}
where $\eta$ regulates the intensity of prioritization, and $S$ represents the dataset. By employing these sampling probabilities, the choice of data samples for each batch is no longer uniform but regulated by their respective rewards. 

The per-instance RL loss, $L(i)$, is computed for the chosen instances, which is then used to optimize the model parameters following the policy gradient theorem. This procedure is formally expressed as 
\begin{equation}
Minimize \; \; E_{i \sim P(i)}[L(i)]
\end{equation}
By continually updating the model based on the most rewarding examples, the PLC bridges the gap between reinforcement learning and supervised learning for sequence prediction tasks. The adaptive nature of the PLC ensures that the model's focus shifts in accordance with the model's evolving knowledge, thereby accelerating the learning process. 

This novel methodology heralds a shift from traditional modes of sequence learning and has the potential to bring about substantial improvements in the efficiency and effectiveness of such models.

\paragraph{Reinforcement Learning Loss}\label{paragraph:more_RL_Loss}

In the context of Reinforcement Learning (RL), we formulate the machine learning task into a Policy Learning problem. The goal of a typical RL agent, often formalized as a policy $\pi$, is to maximize the expected cumulative reward over a series of states $s_t$ and corresponding actions $a_t$:
\[
\pi^* = \underset{\pi}{\operatorname{argmax}} \, \mathbb{E}_{\pi}\left[\sum_{t=0}^{T} r_t\right]
\]
where $r_t$ is the reward at time $t$ and $T$ is the terminal time step. 

Now mapping this RL framework to our sequence learning context, the state $s_t$ can be seen as the input sequence, and the action $a_t$ exemplifies the output sequence, whilst the reward $r_t$ is a signal reflective of how good the predicted sequence is, measured against the target sequence. The better the correspondence between the prediction and the target, the higher the reward. One can argue, the reward can essentially be perceived as being inversely proportional to the Mean Squared Error loss that quantifies this discrepancy:
\[
r = -\frac{1}{N}\sum_{i=1}^{N}(y_i-\hat{y}_i)^2
\]
where $y_i$ is the target sequence, $\hat{y}_i$ is the predicted sequence, and $N$ is the count of the predictions.

This adopting of reinforcement learning parlance thereby innovativeley rephrases the conventional supervised learning problem of finding a set of optimal parameters $\theta$ which minimize the mean squared error loss into a setup geared towards maximizing the expected cumulative reward:

\begin{equation}
\begin{aligned}
\theta^* &= \underset{\theta}{\operatorname{argmax}} \, \mathbb{E}_{\theta}\left[\sum_{t=0}^{T} r_t\right] \\ &= \underset{\theta}{\operatorname{argmin}} \, \mathbb{E}_{\theta}\left[\sum_{t=0}^{T} L(y_t, M(x_t))\right]
\end{aligned}
\end{equation}

where $L$ denotes the MSE loss function, $M$ is the model and $x_t$, $y_t$ are the model inputs and corresponding targets respectively.

The optimal parameters are found by using gradient descent, where the parameters are updated proportionally to the gradient of the expected cumulative reward w.r.t model parameters:

\[
\theta_{t+1} = \theta_t - \alpha \nabla R
\]

where $R$ is the cumulative reward equivalent to $-\sum_{t=0}^{T} L(y_t, M(x_t))$, and $\alpha$ is the learning rate.

This novel perspective not only enriches the mathematical robustness of sequence-to-sequence learning problems but also makes provisions for incorporating clever optimization strategies endemic to reinforcement learning.
