# Supplementary material for: SignLLM: Sign Language Production Large Language Models
Source: arXiv:2405.10718 source file (2025-04-30)
Supplement: Supplementary file 3 [file 3_code.tex]

\begin{algorithm*}
  \SetKwData{Left}{left}\SetKwData{This}{this}\SetKwData{Up}{up}
  \SetKwFunction{Union}{Union}\SetKwFunction{FindCompress}{FindCompress}
  \SetKwInOut{Input}{input}\SetKwInOut{Output}{output}

  \Input{Three arrays $Xx$, $Xy$ and $Xw$ of size $T \times n$, a structure array, a sigma value for noise, a random number generator and a percentile value}
  \Output{Lines array, rootsx, rootsy, rootsz arrays, anglesx, anglesy, anglesz arrays, Yx, Yy, Yz arrays}
  \BlankLine
  \emph{Set T as number of rows and n as number of columns of $Xx$}\;
  
  \emph{Initialize arrays lines, rootsx, rootsy, rootsz, anglesx, anglesy, anglesz}\;
  
  \emph{Set rootsx as first column of $Xx$;Set rootsy as first column of $Xy$}\;
  \emph{Set rootsz as array of zeros with size T}\;
  
  \emph{Add noise to rootsx, rootsy, rootsz arrays}\;
  
  \emph{Initialize arrays Yx, Yy, Yz as arrays of zeros with size $T \times n$}\;
  \emph{Set first column of Yx as rootsx; Set first column of Yy as rootsy; Set first column of Yz as rootsz}\;
  
  \For{each bone in structure}{
    \emph{Add empty list to lines}\;
    \For{each row t in range T}{
      \emph{Compute length L using equation 1}\;
      \emph{Append L to lines}\;
    }
  }
  \For{each line in lines}{
    \emph{Calculate max L as percentile of the line list}\;
    \emph{Assign math.log(max L) to lines array}\;
  }
  
  \For{each bone in structure}{
    \emph{Assign a, b, line as elements of the bone}\;
    \For{each row t in range T}{
      \emph{Compute rotation angles anglex, angley, anglez using equation 2}\;
      \If{any of anglex, angley, anglez is not finite}{
        \emph{Set anglex, angley, anglez as 0.0}\;
      }
      \If{anglez < 0.0}{
        \emph{Set anglez as -anglez}\;
      }
      \emph{Add 0.001 to anglez}\;
      \emph{Normalize anglex, angley, anglez}\;
      \emph{Assign anglex, angley, anglez to anglesx[t, iBone], anglesy[t, iBone], anglesz[t, iBone]}\;
      \emph{Compute new 3D coordinates Yx, Yy, Yz using equation 3}\;
    }
  }
  
  \emph{Reshape rootsx, rootsy, rootsz as arrays of size T $\times$ 1}\;
  
  \emph{Return lines, rootsx, rootsy, rootsz, anglesx, anglesy, anglesz, Yx, Yy, Yz}\;

  %\vspace{12pt}
   \caption{The core formula and code of 2D to 3D conversion.}\label{3_code}
   %\vspace{-12pt}
\end{algorithm*}
%\vspace{-12pt}
