# Supplementary material for: SignLLM: Sign Language Production Large Language Models
Source: arXiv:2405.10718 source file (2025-04-30)
Supplement: Supplementary file 5 [file suppl_cover.tex]

\twocolumn[{%
\renewcommand\twocolumn[1][]{#1}%
\maketitlesupplementary
\begin{center}
    \centering
    \includegraphics[width=.99\textwidth]{fig/cover_old.drawio.png}
    \captionof{figure}{\textbf{Bilingual Sign Language Production:} (a) Enter an American English or German sentence you want to translate; (b) Our \ourLLMmethodName{} then translates the text into a continuous skeleton pose sequence, and supports prompt word input; (c) The textual correspondence of sign language skeletal postures varies across different countries. These postures can be post-processed into more comprehensible images via conditional image generation models such as ControlNet.
    %Skeletal postures for sign language, which vary among different countries, can be subsequently processed by Conditional Control Image Generation Models like ControlNet.
    }
    \label{fig:cover_old}
\end{center}
}]
