# Supplementary material for: SignLLM: Sign Language Production Large Language Models
Source: arXiv:2405.10718 source file (2025-04-30)
Supplement: Supplementary file 6 [file prompt.tex]

\begin{table}[h]
\caption{\textbf{Prompt Ablation Study:} We added a row of comparative data to the table, $T$ represents a model that uses Text2LangGloss, but does not use Prompt as input this time.}
\label{tab:prompt_supp}
\centering
\resizebox{0.99\linewidth}{!}{%
\begin{tabular}{@{}p{3.0cm}ccccc@{}}
\toprule
     & \multicolumn{2}{c}{DEV SET}  & \multicolumn{2}{c}{TEST SET} \\
\multicolumn{1}{c}{Approach:}  & \multicolumn{1}{c}{BLEU-4 $\uparrow$} & \multicolumn{1}{c}{ROUGE $\uparrow$} & \multicolumn{1}{c}{BLEU-4 $\uparrow$} & \multicolumn{1}{c}{ROUGE $\uparrow$} \\ \midrule
\multicolumn{1}{r|}{Baseline \cite{stoll2018sign}} & 16.34 & 48.42 & 15.26 & 48.10 \\
\multicolumn{1}{r|}{Stoll et al. \cite{saunders2020progressive}} & 20.23 & 55.41 & 19.10 & 54.55 \\
\multicolumn{1}{r|}{\textbf{T (no prompt)}} & \textbf{22.45} & \textbf{53.56} & \textbf{20.12} & \textbf{51.37} \\
\multicolumn{1}{r|}{\textbf{Ours}} & \textbf{23.10} & \textbf{58.76} & \textbf{22.05} & \textbf{56.46} \\
\bottomrule
\end{tabular}%
}
% \vspace{}
\vspace{-14pt}
\end{table}
