# Supplementary material for: SignLLM: Sign Language Production Large Language Models
Source: arXiv:2405.10718 source file (2025-04-30)
Supplement: Supplementary file 7 [file prompt_temp_short.tex]

% \begin{table*}[p]
%     \centering
%     \begin{tabularx}{\textwidth}{|X|}
%     \hline
%         \textbf{Prompt Template \& Some Examples} \hline
% & ~ \textbf{Part I}\\
% I really want to learn how to say ``\{\texttt{Text}\}'' in sign language. Can you help me?\\
% How would you express ``\{\texttt{Text}\}'' in sign language?\\
% Can you show me how to say ``\{\texttt{Text}\}'' in sign language?\\
% How do I say ``\{\texttt{Text}\}'' in sign language?\\ 
% Could you tell me how ``\{\texttt{Text}\}'' is represented in sign language?\\
% What is the sign language for ``\{\texttt{Text}\}''?& ~  \hline
% & ~ \textbf{Part II}\\
% How is ``So we're going to go up and down; let's switch hands, down and up; down and up.'' denoted in sign language?\\
% Can you elucidate how And just let those fingers relax. looks in sign language?\\
% I really want to learn how Now together you're going to go opposite. is said in sign language. Can you help?\\
% How do I articulate ``It's real easy to actually get your fingers to lead, so try not to let them do that.'' using sign language?\\
% I am intrigued to learn the sign language for `Let the wrist do all the leading.'.\\
% I am wondering how ``Don't let the fingers take over, let the wrist do all the guiding.'' appears in sign language. & ~  \hline
% & ~ \textbf{Part III}\\
% Ich möchte wirklich lernen wie man ``\{\texttt{Text}\}'' in Gebärdensprache sagt. Können Sie mir helfen?\\
% Wie würden Sie ``\{\texttt{Text}\}'' in Gebärdensprache ausdrücken?\\
% Können Sie mir zeigen wie man ``\{\texttt{Text}\}'' mit Gebärdensprache sagt?\\
% Wie sage ich ``\{\texttt{Text}\}'' in Gebärdensprache?\\
% Könnten Sie mir sagen wie ``\{\texttt{Text}\}'' in Gebärdensprache dargestellt wird?\\
% Was ist die Gebärdensprache für ``\{\texttt{Text}\}''? & ~  \hline
% & ~ \textbf{Part IV}\\
% 'regen und schnee lassen an den alpen in der nacht nach im norden und nordosten fallen hier und da schauer sonst ist das klar' Wie stellt man das in Gebärdensprache dar?\\
% %Können Sie die Gebärdensprache für 'am donnerstag regen in der nordhälfte in der südhälfte mal sonne mal wolken ähnliches wetter dann auch am freitag' demonstrieren?\\
% %Mich interessiert, wie vom nordmeer zieht ein kräftiges tief heran und bringt uns ab den morgenstunden heftige schneefälle zum teil auch gefrierenden regen in Gebärdensprache aussieht.\\
% Wie wird sonnig geht es auch ins wochenende samstag ein herrlicher tag mit temperaturen bis siebzehn grad hier im westen in Gebärdensprache dargestellt?\\
% Wie würden Sie deutschland liegt morgen unter hochdruckeinfluss der die wolken weitgehend vertreibt gebärden?\\
% Können Sie mir zeigen, wie am sonntag im nordwesten eine mischung aus sonne und wolken mit einigen zum teil gewittrigen schauern in Gebärdensprache aussieht?\\
% Wie sieht die Gebärdensprache für örtlich schauer oder gewitter die heftig sein können aus?\\
% Was ist die Gebärdensprache für und zum wochenende wird es dann sogar wieder ein bisschen kälter? & ~  \hline
%     \end{tabularx}
%     %\vspace{-4pt}
%     \caption{We provide two templates for sign language as a reference, and \texttt{\{Text\}} is where the video oral dialogue is inserted.}
%     %\vspace{-12pt}
%     \label{tab:temp_supp}
% \end{table*}

\begin{table*}[p]
    \centering
    \begin{tabularx}{\textwidth}{|X|} % Correct column specification
    \hline
    \textbf{Prompt Template \& Some Examples} \\ \hline
    \textbf{Part I} \\ \hline
    I really want to learn how to say ``\{\texttt{Text}\}'' in sign language. Can you help me? \\ \hline
    How would you express ``\{\texttt{Text}\}'' in sign language? \\ \hline
    Can you show me how to say ``\{\texttt{Text}\}'' in sign language? \\ \hline
    How do I say ``\{\texttt{Text}\}'' in sign language? \\ \hline
    Could you tell me how ``\{\texttt{Text}\}'' is represented in sign language? \\ \hline
    What is the sign language for ``\{\texttt{Text}\}''? \\ \hline
    \textbf{Part II} \\ \hline
    How is ``So we're going to go up and down; let's switch hands, down and up; down and up.'' denoted in sign language? \\ \hline
    Can you elucidate how ``And just let those fingers relax.'' looks in sign language? \\ \hline
    I really want to learn how ``Now together you're going to go opposite.'' is said in sign language. Can you help? \\ \hline
    How do I articulate ``It's real easy to actually get your fingers to lead, so try not to let them do that.'' using sign language? \\ \hline
    I am intrigued to learn the sign language for ``Let the wrist do all the leading.'' \\ \hline
    I am wondering how ``Don't let the fingers take over, let the wrist do all the guiding.'' appears in sign language. \\ \hline
    \textbf{Part III} \\ \hline
    Ich möchte wirklich lernen wie man ``\{\texttt{Text}\}'' in Gebärdensprache sagt. Können Sie mir helfen? \\ \hline
    Wie würden Sie ``\{\texttt{Text}\}'' in Gebärdensprache ausdrücken? \\ \hline
    Können Sie mir zeigen wie man ``\{\texttt{Text}\}'' mit Gebärdensprache sagt? \\ \hline
    Wie sage ich ``\{\texttt{Text}\}'' in Gebärdensprache? \\ \hline
    Könnten Sie mir sagen wie ``\{\texttt{Text}\}'' in Gebärdensprache dargestellt wird? \\ \hline
    Was ist die Gebärdensprache für ``\{\texttt{Text}\}''? \\ \hline
    \textbf{Part IV} \\ \hline
    'Regen und Schnee lassen an den Alpen in der Nacht nach, im Norden und Nordosten fallen hier und da Schauer, sonst ist das klar' Wie stellt man das in Gebärdensprache dar? \\ \hline
    %Können Sie die Gebärdensprache für 'am Donnerstag Regen in der Nordhälfte, in der Südhälfte mal Sonne mal Wolken, ähnliches Wetter dann auch am Freitag' demonstrieren? \\ \hline
    %Mich interessiert, wie 'vom Nordmeer zieht ein kräftiges Tief heran und bringt uns ab den Morgenstunden heftige Schneefälle, zum Teil auch gefrierenden Regen' in Gebärdensprache aussieht. \\ \hline
    Wie wird 'Sonnig geht es auch ins Wochenende, Samstag ein herrlicher Tag mit Temperaturen bis siebzehn Grad hier im Westen' in Gebärdensprache dargestellt? \\ \hline
    Wie würden Sie 'Deutschland liegt morgen unter Hochdruckeinfluss, der die Wolken weitgehend vertreibt' gebärden? \\ \hline
    Können Sie mir zeigen, wie 'am Sonntag im Nordwesten eine Mischung aus Sonne und Wolken mit einigen zum Teil gewittrigen Schauern' in Gebärdensprache aussieht? \\ \hline
    Wie sieht die Gebärdensprache für 'örtlich Schauer oder Gewitter, die heftig sein können' aus? \\ \hline
    Was ist die Gebärdensprache für 'und zum Wochenende wird es dann sogar wieder ein bisschen kälter'? \\ \hline
    \end{tabularx}
    %\vspace{-4pt}
    \caption{We provide two templates for sign language as a reference, and \texttt{\{Text\}} is where the video oral dialogue is inserted.}
    %\vspace{-12pt}
    \label{tab:temp_supp}
\end{table*}
